# Supplementary material for: Model Slicing for Supporting Complex Analytics with Elastic Inference Cost and Resource Constraints
Source: arXiv:1904.01831 source file (2021-04-21)
Supplement: Supplementary file 1 [file appendix.tex]

\section{Appendix}

\begin{table*}[h!]
    \centering
    
    \caption{Remaining estimated percentage of 
    % memory ($M_t$) and 
    computation footprint ($C_t$), error rate of VGG-13 on CIFAR-10 with different lower bounds w.r.t slice rate $r$. Results that surpass other lower bound networks are underlined with \textbf{Bold} font. Results of lower bond networks sliced under the same slice rate are in \textbf{Bold} \textit{Italic} font.}
    \resizebox{2\columnwidth}{!}{
        \begin{tabular}{ c || c|cc|cc|cc|cc|cc|cc}
    \thickhline
    Slice Rate $\mathbf{r}$ & 1.000 & 0.9375 & 0.8750 & 0.8125 & 0.7500  & 0.6875 & 0.6250 & 0.5625 & 0.500 & 0.4375 & 0.375 & 0.3125 & 0.2500  \\
    % \hline
    % $\mathbf{M_t}$  & 100.0\% & 93.75\%  & 87.50\% & 81.25\% & 75.00\% & 68.75\% & 62.50\% & 56.25\% & 50.00\% & 43.75\% & 37.50\% & 31.25\% & 25.00\% \\
    % % \hline
    $\mathbf{C_t}$  & 100.0\% & 87.89\%  & 76.56\% & 66.02\% & 56.25\% & 47.27\% & 39.06\% & 31.64\% & 25.00\% & 19.14\% & 14.06\% & 9.77\% & 6.25\% \\
    \hline
    lb 0.2500  & 6.19 & 6.29 & 6.28 & 6.37 & 6.48 & 6.80 & 7.13 & 7.38 & 8.09 & 9.46 & 10.79 & \underline{\textbf{13.93}} & \underline{\textit{\textbf{17.04}}} \\
    lb 0.3750  & 5.65 & \textbf{\underline{5.80}} & \textbf{\underline{5.84}} & \textbf{\underline{5.87}} & \textbf{\underline{5.78}} & \textbf{\underline{5.91}} & \textbf{\underline{6.12}} & \textbf{\underline{6.68}} & \textbf{\underline{7.44}} & \textbf{\underline{7.74}} & \textbf{\textit{\underline{8.62}}} & 28.14 & 65.23 \\
    lb 0.5000  & 6.03 & 6.03 & 6.04 & 6.11 & 6.33 & 6.57 & 6.83 & 7.08 & \textbf{\textit{7.64}} & 17.76 & 41.68 & 65.50 & 78.06 \\
    lb 0.6250  & 6.08 & 6.07 & 6.11 & 6.25 & 6.38 & 6.60 & \textit{\textbf{6.60}} & 13.73 & 27.98 & 53.32 & 85.42 & 89.90 & 89.57 \\
    lb 0.7500  & 5.96 & 5.96 & 5.93 & 6.02 & \textbf{\textit{6.22}} & 10.40 & 21.19 & 41.65 & 59.89 & 65.98 & 88.66 & 88.49 & 89.99 \\
    lb 0.8750  & 6.15 & 6.15 & \textbf{\textit{6.16}} & 8.26 & 14.39 & 20.55 & 33.45 & 45.00 & 65.24 & 81.45 & 84.72 & 86.49 & 88.38 \\
    lb 1.0000  & \textbf{\textit{\underline{5.49}}} & 8.11 & 12.45 & 18.37 & 32.07 & 42.04 & 55.82 & 73.09 & 78.63 & 83.65 & 87.77 & 89.73 & 89.81 \\
    \thickhline
        \end{tabular}
    }%\vspace{+0.2cm}
    \label{tab:lb_table}
\end{table*}

\subsection{Residual Learning in \TopicWord[M][S]}
\label{sec:residual_learning_effect}

Our \textit{\TopicWord} training scheme structurally is reminiscent of residual learning proposed in ResNet~\cite{he2016deep,he2016identity}.
In ResNet, a shortcut connection of identity mapping is proposed to forward input to output directly: $\mathbf{Y} = \mathcal{F}_{conv}(\mathbf{X}) + \mathbf{X}$, where during optimization, the convolutional transformation only needs to learn the residual representation on top of input information $\mathbf{X}$, namely $\mathbf{Y}-\mathbf{X}$.
Analogously, networks trained with \TopicWord[M][S] learn to accumulate the representation with additional basic components introduced, specifically neurons in dense layers and channels in convolutional layers.

\begin{figure}[h!]
    \centering
        \includegraphics[width=0.45\textwidth]{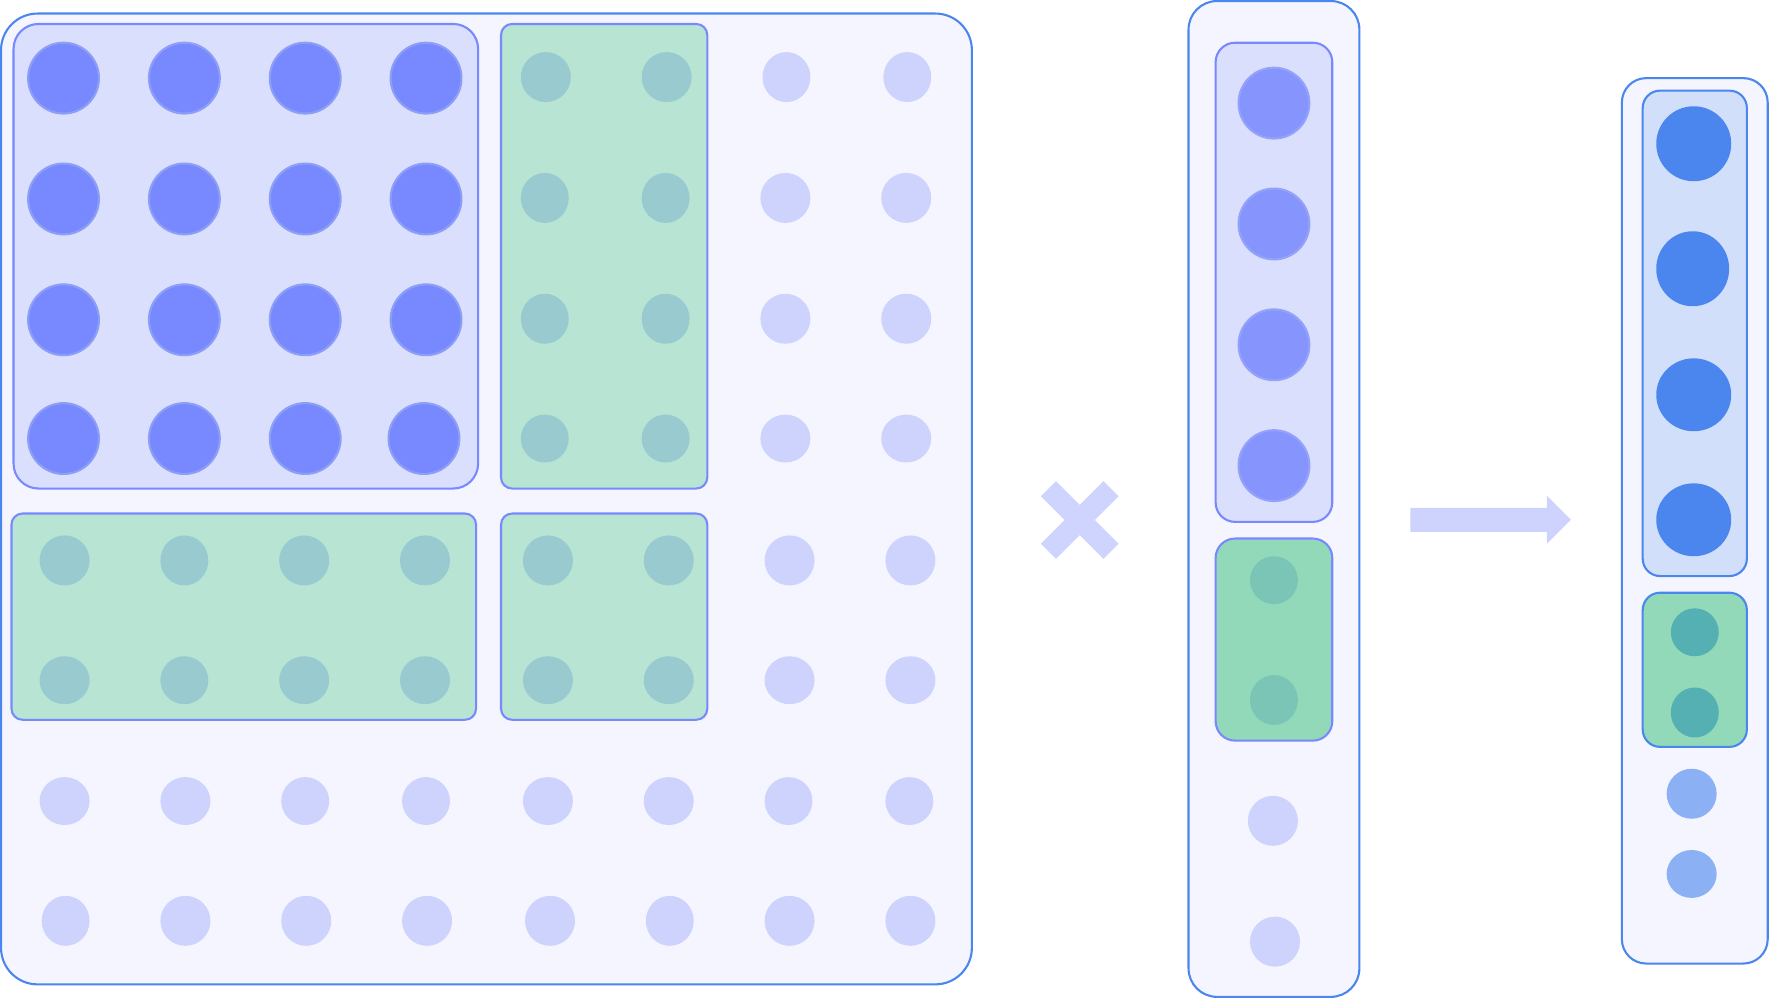}
    \caption{Illustration of the residual learning in \textit{\TopicWord}, where the representation can be built up progressively with minimum additional cost.}
    \label{fig:multiplication_residual}
\end{figure}

To demonstrate the residual learning effect in \textit{\TopicWord}, we take the transformation in a fully connected layer for example, and analyze the relationship between any two sub-layers of \textit{slice rate} $r_1$ and $r_2$ with $r_1 < r_2$.
As is illustrated in Figure~\ref{fig:multiplication_residual}, we have the transformation of the $r_1$-layer as $\mathbf{Y}_1 = \mathbf{W}_1 \mathbf{X}_1$ and the transformation of the $r_2$-layer $[\mathbf{\tilde{Y}}_1; \mathbf{Y}_2] = \mathbf{W}_2 [\mathbf{X}_1; \mathbf{X}_2]$ in block matrix multiplication as:

\begin{gather}
    \begin{bmatrix} \mathbf{\tilde{Y}}_1 \\ \mathbf{Y}_2 \end{bmatrix} =
    \begin{bmatrix}
    \mathbf{W}_1 & \mathbf{B} \\
    \mathbf{C} & \mathbf{D}
    \end{bmatrix} \cdot
    \begin{bmatrix}
    \mathbf{X}_1 \\ \mathbf{X}_2
    \end{bmatrix} =
    \begin{bmatrix}
    \mathbf{W}_1 \mathbf{X}_1 + \mathbf{B} \mathbf{X}_2 \\
    \mathbf{C} \mathbf{X}_1 + \mathbf{D} \mathbf{X}_2
    \end{bmatrix}
\end{gather}

Here, $\mathbf{X}_2$ is the additional input introduced for $r_2$-layer and $\mathbf{Y}_2$ the corresponding supplementary output produced.
Suppose $r_2-r_1 \ll r_1$, which generally holds true, then the residual learning representation can be clarified in two angles.
Firstly, the base representation of $r_2$-layer $\mathbf{\tilde{Y}}_1 = \mathbf{W}_1 \mathbf{X}_1 + \mathbf{B} \mathbf{X}_2 = \mathbf{Y}_1 + \mathbf{B} \mathbf{X}_2$, which is composed of the base representation $\mathbf{Y}_1$ and the residual representation $\mathbf{B} \mathbf{X}_2$.
Secondly, the output $\mathbf{Y}_2$ also forms the residual representation in another dimension that is supplementary to the base representation $\mathbf{\tilde{Y}}_1$ in the $r_2$ layer.

The justification for the residual learning effect is that the base representation of $\mathbf{Y}_1$ in $r_1$-layer is already optimized for the learning task as the training progresses.
Therefore, the additional representation introduced to $r_2$-layer evolves to form the residual representation, as is corroborated in the visualization in Section~\ref{visualization}.
Furthermore, this residual learning characteristic provides an efficient way to harness the finer representation of $r_2$-net based on $r_1$-net by the simple approximation of $\mathbf{\tilde{Y}}_1 \approx  \mathbf{Y}_1$.
With this approximation in every layer of the network, the most computationally heavy features of $\mathbf{W}_1 \mathbf{X}_1$ can be reused without re-evaluating, thus the representation of $r_2$-layer can be updated by calculating $\mathbf{C} \mathbf{X}_1 + \mathbf{D} \mathbf{X}_2$ with orders of magnitude lower computational cost.
